# Supplementary material for: TabPack: Efficient Hyperparameter Ensembles for Tabular Deep Learning
Source: arXiv:2607.05380 source file (2026-07-06)
Supplement: Supplementary file 1 [file appendix_independent.tex]

\newcommand{\topalign}[1]{%
\vtop{\vskip 0pt #1}}

\begin{longtable}{p{0.3\textwidth}p{0.3\textwidth}p{0.3\textwidth}}
\caption{Extended results (mean $\pm$ std of the metric on the test set) for the main benchmark. Results are grouped by datasets. \textuparrow\ corresponds to either accuracy or ROC-AUC depending on a classification dataset. \textdownarrow\ corresponds to RMSE on regression datasets.}\\

\topalign{
\setlength\tabcolsep{2.5pt}

\begin{tabular}{lll}

\multicolumn{2}{c}{Churn \textuparrow} \\
\toprule
Method & Single model \\
\midrule\\[-0.45cm]
{\footnotesize $\mathrm{MLP}$ } & {\footnotesize$0.8562 \pm 0.0018$} \\ 
{\footnotesize $\mathrm{TabPack}$ } & {\footnotesize$0.8581 \pm 0.0029$} \\ 
{\footnotesize $\mathrm{MLP^\dagger}$ } & {\footnotesize$0.8633 \pm 0.0029$} \\ 
{\footnotesize $\mathrm{XGBoost}$ } & {\footnotesize$0.8605 \pm 0.0020$} \\ 
{\footnotesize $\mathrm{TabM}$ } & {\footnotesize$0.8638 \pm 0.0017$} \\ 
{\footnotesize MLP$_\text{HPE}^\dagger$ } & {\footnotesize$0.8613 \pm 0.0015$} \\ 
{\footnotesize $\mathrm{\method_\text{Offline}^\dagger}$ } & {\footnotesize$0.8588 \pm 0.0049$} \\ 
{\footnotesize $\mathrm{TabM^\dagger}$ } & {\footnotesize$0.8609 \pm 0.0014$} \\ 
{\footnotesize $\mathrm{TabPack^\dagger}$ } & {\footnotesize$0.8623 \pm 0.0028$} \\ 
\bottomrule
\end{tabular}}

&

\topalign{
\setlength\tabcolsep{2.5pt}

\begin{tabular}{lll}

\multicolumn{2}{c}{California \textdownarrow} \\
\toprule
Method & Single model \\
\midrule\\[-0.45cm]
{\footnotesize $\mathrm{MLP}$ } & {\footnotesize$0.4819 \pm 0.0023$} \\ 
{\footnotesize $\mathrm{TabPack}$ } & {\footnotesize$0.4710 \pm 0.0014$} \\ 
{\footnotesize $\mathrm{MLP^\dagger}$ } & {\footnotesize$0.4376 \pm 0.0022$} \\ 
{\footnotesize $\mathrm{XGBoost}$ } & {\footnotesize$0.4329 \pm 0.0011$} \\ 
{\footnotesize $\mathrm{TabM}$ } & {\footnotesize$0.4324 \pm 0.0026$} \\ 
{\footnotesize MLP$_\text{HPE}^\dagger$ } & {\footnotesize$0.4232 \pm 0.0021$} \\ 
{\footnotesize $\mathrm{\method_\text{Offline}^\dagger}$ } & {\footnotesize$0.4203 \pm 0.0028$} \\ 
{\footnotesize $\mathrm{TabM^\dagger}$ } & {\footnotesize$0.4028 \pm 0.0019$} \\ 
{\footnotesize $\mathrm{TabPack^\dagger}$ } & {\footnotesize$0.4176 \pm 0.0028$} \\ 
\bottomrule
\end{tabular}}

&

\topalign{
\setlength\tabcolsep{2.5pt}

\begin{tabular}{lll}

\multicolumn{2}{c}{House \textdownarrow} \\
\toprule
Method & Single model \\
\midrule\\[-0.45cm]
{\footnotesize $\mathrm{MLP}$ } & {\footnotesize$30387.3601 \pm 214.1497$} \\ 
{\footnotesize $\mathrm{TabPack}$ } & {\footnotesize$29724.4199 \pm 184.4139$} \\ 
{\footnotesize $\mathrm{MLP^\dagger}$ } & {\footnotesize$29851.0959 \pm 411.2211$} \\ 
{\footnotesize $\mathrm{XGBoost}$ } & {\footnotesize$31380.6797 \pm 60.4100$} \\ 
{\footnotesize $\mathrm{TabM}$ } & {\footnotesize$30389.6157 \pm 123.6157$} \\ 
{\footnotesize MLP$_\text{HPE}^\dagger$ } & {\footnotesize$29508.1265 \pm 34.5536$} \\ 
{\footnotesize $\mathrm{\method_\text{Offline}^\dagger}$ } & {\footnotesize$29538.1678 \pm 332.2177$} \\ 
{\footnotesize $\mathrm{TabM^\dagger}$ } & {\footnotesize$30151.1698 \pm 217.8215$} \\ 
{\footnotesize $\mathrm{TabPack^\dagger}$ } & {\footnotesize$29548.6146 \pm 174.7837$} \\ 
\bottomrule
\end{tabular}}

\\

\topalign{
\setlength\tabcolsep{2.5pt}

\begin{tabular}{lll}

\multicolumn{2}{c}{Adult \textuparrow} \\
\toprule
Method & Single model \\
\midrule\\[-0.45cm]
{\footnotesize $\mathrm{MLP}$ } & {\footnotesize$0.8561 \pm 0.0012$} \\ 
{\footnotesize $\mathrm{TabPack}$ } & {\footnotesize$0.8571 \pm 0.0012$} \\ 
{\footnotesize $\mathrm{MLP^\dagger}$ } & {\footnotesize$0.8692 \pm 0.0018$} \\ 
{\footnotesize $\mathrm{XGBoost}$ } & {\footnotesize$0.8709 \pm 0.0007$} \\ 
{\footnotesize $\mathrm{TabM}$ } & {\footnotesize$0.8577 \pm 0.0007$} \\ 
{\footnotesize MLP$_\text{HPE}^\dagger$ } & {\footnotesize$0.8680 \pm 0.0012$} \\ 
{\footnotesize $\mathrm{\method_\text{Offline}^\dagger}$ } & {\footnotesize$0.8679 \pm 0.0030$} \\ 
{\footnotesize $\mathrm{TabM^\dagger}$ } & {\footnotesize$0.8674 \pm 0.0010$} \\ 
{\footnotesize $\mathrm{TabPack^\dagger}$ } & {\footnotesize$0.8693 \pm 0.0007$} \\ 
\bottomrule
\end{tabular}}

&

\topalign{
\setlength\tabcolsep{2.5pt}

\begin{tabular}{lll}

\multicolumn{2}{c}{Diamond \textdownarrow} \\
\toprule
Method & Single model \\
\midrule\\[-0.45cm]
{\footnotesize $\mathrm{MLP}$ } & {\footnotesize$0.1359 \pm 0.0012$} \\ 
{\footnotesize $\mathrm{TabPack}$ } & {\footnotesize$0.1329 \pm 0.0003$} \\ 
{\footnotesize $\mathrm{MLP^\dagger}$ } & {\footnotesize$0.1343 \pm 0.0008$} \\ 
{\footnotesize $\mathrm{XGBoost}$ } & {\footnotesize$0.1337 \pm 0.0004$} \\ 
{\footnotesize $\mathrm{TabM}$ } & {\footnotesize$0.1315 \pm 0.0010$} \\ 
{\footnotesize MLP$_\text{HPE}^\dagger$ } & {\footnotesize$0.1309 \pm 0.0003$} \\ 
{\footnotesize $\mathrm{\method_\text{Offline}^\dagger}$ } & {\footnotesize$0.1304 \pm 0.0008$} \\ 
{\footnotesize $\mathrm{TabM^\dagger}$ } & {\footnotesize$0.1306 \pm 0.0007$} \\ 
{\footnotesize $\mathrm{TabPack^\dagger}$ } & {\footnotesize$0.1307 \pm 0.0007$} \\ 
\bottomrule
\end{tabular}}

&

\topalign{
\setlength\tabcolsep{2.5pt}

\begin{tabular}{lll}

\multicolumn{2}{c}{Otto \textuparrow} \\
\toprule
Method & Single model \\
\midrule\\[-0.45cm]
{\footnotesize $\mathrm{MLP}$ } & {\footnotesize$0.8218 \pm 0.0029$} \\ 
{\footnotesize $\mathrm{TabPack}$ } & {\footnotesize$0.8232 \pm 0.0019$} \\ 
{\footnotesize $\mathrm{MLP^\dagger}$ } & {\footnotesize$0.8237 \pm 0.0023$} \\ 
{\footnotesize $\mathrm{XGBoost}$ } & {\footnotesize$0.8301 \pm 0.0016$} \\ 
{\footnotesize $\mathrm{TabM}$ } & {\footnotesize$0.8278 \pm 0.0012$} \\ 
{\footnotesize MLP$_\text{HPE}^\dagger$ } & {\footnotesize$0.8240 \pm 0.0025$} \\ 
{\footnotesize $\mathrm{\method_\text{Offline}^\dagger}$ } & {\footnotesize$0.8254 \pm 0.0024$} \\ 
{\footnotesize $\mathrm{TabM^\dagger}$ } & {\footnotesize$0.8332 \pm 0.0021$} \\ 
{\footnotesize $\mathrm{TabPack^\dagger}$ } & {\footnotesize$0.8281 \pm 0.0017$} \\ 
\bottomrule
\end{tabular}}

\\

\topalign{
\setlength\tabcolsep{2.5pt}

\begin{tabular}{lll}

\multicolumn{2}{c}{Higgs-Small \textuparrow} \\
\toprule
Method & Single model \\
\midrule\\[-0.45cm]
{\footnotesize $\mathrm{MLP}$ } & {\footnotesize$0.7267 \pm 0.0013$} \\ 
{\footnotesize $\mathrm{TabPack}$ } & {\footnotesize$0.7294 \pm 0.0015$} \\ 
{\footnotesize $\mathrm{MLP^\dagger}$ } & {\footnotesize$0.7279 \pm 0.0007$} \\ 
{\footnotesize $\mathrm{XGBoost}$ } & {\footnotesize$0.7271 \pm 0.0009$} \\ 
{\footnotesize $\mathrm{TabM}$ } & {\footnotesize$0.7409 \pm 0.0029$} \\ 
{\footnotesize MLP$_\text{HPE}^\dagger$ } & {\footnotesize$0.7302 \pm 0.0010$} \\ 
{\footnotesize $\mathrm{\method_\text{Offline}^\dagger}$ } & {\footnotesize$0.7299 \pm 0.0004$} \\ 
{\footnotesize $\mathrm{TabM^\dagger}$ } & {\footnotesize$0.7352 \pm 0.0008$} \\ 
{\footnotesize $\mathrm{TabPack^\dagger}$ } & {\footnotesize$0.7317 \pm 0.0010$} \\ 
\bottomrule
\end{tabular}}

&

\topalign{
\setlength\tabcolsep{2.5pt}

\begin{tabular}{lll}

\multicolumn{2}{c}{Black-Friday \textdownarrow} \\
\toprule
Method & Single model \\
\midrule\\[-0.45cm]
{\footnotesize $\mathrm{MLP}$ } & {\footnotesize$0.6927 \pm 0.0006$} \\ 
{\footnotesize $\mathrm{TabPack}$ } & {\footnotesize$0.6871 \pm 0.0001$} \\ 
{\footnotesize $\mathrm{MLP^\dagger}$ } & {\footnotesize$0.6816 \pm 0.0006$} \\ 
{\footnotesize $\mathrm{XGBoost}$ } & {\footnotesize$0.6808 \pm 0.0001$} \\ 
{\footnotesize $\mathrm{TabM}$ } & {\footnotesize$0.6846 \pm 0.0003$} \\ 
{\footnotesize MLP$_\text{HPE}^\dagger$ } & {\footnotesize$0.6798 \pm 0.0007$} \\ 
{\footnotesize $\mathrm{\method_\text{Offline}^\dagger}$ } & {\footnotesize$0.6799 \pm 0.0002$} \\ 
{\footnotesize $\mathrm{TabM^\dagger}$ } & {\footnotesize$0.6766 \pm 0.0006$} \\ 
{\footnotesize $\mathrm{TabPack^\dagger}$ } & {\footnotesize$0.6784 \pm 0.0002$} \\ 
\bottomrule
\end{tabular}}

&

\topalign{
\setlength\tabcolsep{2.5pt}

\begin{tabular}{lll}

\multicolumn{2}{c}{Microsoft \textdownarrow} \\
\toprule
Method & Single model \\
\midrule\\[-0.45cm]
{\footnotesize $\mathrm{MLP}$ } & {\footnotesize$0.7455 \pm 0.0003$} \\ 
{\footnotesize $\mathrm{TabPack}$ } & {\footnotesize$0.7423 \pm 0.0001$} \\ 
{\footnotesize $\mathrm{MLP^\dagger}$ } & {\footnotesize$0.7447 \pm 0.0002$} \\ 
{\footnotesize $\mathrm{XGBoost}$ } & {\footnotesize$0.7412 \pm 0.0001$} \\ 
{\footnotesize $\mathrm{TabM}$ } & {\footnotesize$0.7422 \pm 0.0004$} \\ 
{\footnotesize MLP$_\text{HPE}^\dagger$ } & {\footnotesize$0.7423 \pm 0.0003$} \\ 
{\footnotesize $\mathrm{\method_\text{Offline}^\dagger}$ } & {\footnotesize$0.7420 \pm 0.0002$} \\ 
{\footnotesize $\mathrm{TabM^\dagger}$ } & {\footnotesize$0.7407 \pm 0.0002$} \\ 
{\footnotesize $\mathrm{TabPack^\dagger}$ } & {\footnotesize$0.7395 \pm 0.0002$} \\ 
\bottomrule
\end{tabular}}

\end{longtable}
