# Supplementary material for: TabPack: Efficient Hyperparameter Ensembles for Tabular Deep Learning
Source: arXiv:2607.05380 source file (2026-07-06)
Supplement: Supplementary file 2 [file appendix_tabred.tex]

\begin{longtable}{p{0.3\textwidth}p{0.3\textwidth}p{0.3\textwidth}}
\caption{Extended results for the main benchmark. Results are grouped by datasets. The notation follows that of the previous table.}\\

\topalign{
\setlength\tabcolsep{2.5pt}

\begin{tabular}{lll}

\multicolumn{2}{c}{Sberbank-Housing \textdownarrow} \\
\toprule
Method & Single model \\
\midrule\\[-0.45cm]
{\footnotesize $\mathrm{MLP}$ } & {\footnotesize$0.2608 \pm 0.0149$} \\ 
{\footnotesize $\mathrm{TabPack}$ } & {\footnotesize$0.2419 \pm 0.0011$} \\ 
{\footnotesize $\mathrm{MLP^\dagger}$ } & {\footnotesize$0.2481 \pm 0.0038$} \\ 
{\footnotesize $\mathrm{XGBoost}$ } & {\footnotesize$0.2407 \pm 0.0004$} \\ 
{\footnotesize $\mathrm{TabM}$ } & {\footnotesize$0.2424 \pm 0.0033$} \\ 
{\footnotesize MLP$_\text{HPE}^\dagger$ } & {\footnotesize$0.2336 \pm 0.0004$} \\ 
{\footnotesize $\mathrm{\method_\text{Offline}^\dagger}$ } & {\footnotesize$0.2307 \pm 0.0005$} \\ 
{\footnotesize $\mathrm{TabM^\dagger}$ } & {\footnotesize$0.2343 \pm 0.0013$} \\ 
{\footnotesize $\mathrm{TabPack^\dagger}$ } & {\footnotesize$0.2302 \pm 0.0014$} \\ 
\bottomrule
\end{tabular}}

&

\topalign{
\setlength\tabcolsep{2.5pt}

\begin{tabular}{lll}

\multicolumn{2}{c}{Ecom-Offers \textuparrow} \\
\toprule
Method & Single model \\
\midrule\\[-0.45cm]
{\footnotesize $\mathrm{MLP}$ } & {\footnotesize$0.6011 \pm 0.0025$} \\ 
{\footnotesize $\mathrm{TabPack}$ } & {\footnotesize$0.6007 \pm 0.0014$} \\ 
{\footnotesize $\mathrm{MLP^\dagger}$ } & {\footnotesize$0.5993 \pm 0.0008$} \\ 
{\footnotesize $\mathrm{XGBoost}$ } & {\footnotesize$0.5741 \pm 0.0055$} \\ 
{\footnotesize $\mathrm{TabM}$ } & {\footnotesize$0.6016 \pm 0.0004$} \\ 
{\footnotesize MLP$_\text{HPE}^\dagger$ } & {\footnotesize$0.5983 \pm 0.0002$} \\ 
{\footnotesize $\mathrm{\method_\text{Offline}^\dagger}$ } & {\footnotesize$0.5979 \pm 0.0007$} \\ 
{\footnotesize $\mathrm{TabM^\dagger}$ } & {\footnotesize$0.5984 \pm 0.0010$} \\ 
{\footnotesize $\mathrm{TabPack^\dagger}$ } & {\footnotesize$0.5989 \pm 0.0017$} \\ 
\bottomrule
\end{tabular}}

&

\topalign{
\setlength\tabcolsep{2.5pt}

\begin{tabular}{lll}

\multicolumn{2}{c}{Maps-Routing \textdownarrow} \\
\toprule
Method & Single model \\
\midrule\\[-0.45cm]
{\footnotesize $\mathrm{MLP}$ } & {\footnotesize$0.1622 \pm 0.0001$} \\ 
{\footnotesize $\mathrm{TabPack}$ } & {\footnotesize$0.1612 \pm 0.0000$} \\ 
{\footnotesize $\mathrm{MLP^\dagger}$ } & {\footnotesize$0.1612 \pm 0.0001$} \\ 
{\footnotesize $\mathrm{XGBoost}$ } & {\footnotesize$0.1618 \pm 0.0000$} \\ 
{\footnotesize $\mathrm{TabM}$ } & {\footnotesize$0.1611 \pm 0.0001$} \\ 
{\footnotesize MLP$_\text{HPE}^\dagger$ } & {\footnotesize$0.1606 \pm 0.0000$} \\ 
{\footnotesize $\mathrm{\method_\text{Offline}^\dagger}$ } & {\footnotesize$0.1606 \pm 0.0000$} \\ 
{\footnotesize $\mathrm{TabM^\dagger}$ } & {\footnotesize$0.1606 \pm 0.0002$} \\ 
{\footnotesize $\mathrm{TabPack^\dagger}$ } & {\footnotesize$0.1605 \pm 0.0001$} \\ 
\bottomrule
\end{tabular}}

\\

\topalign{
\setlength\tabcolsep{2.5pt}

\begin{tabular}{lll}

\multicolumn{2}{c}{Homesite-Insurance \textuparrow} \\
\toprule
Method & Single model \\
\midrule\\[-0.45cm]
{\footnotesize $\mathrm{MLP}$ } & {\footnotesize$0.9515 \pm 0.0007$} \\ 
{\footnotesize $\mathrm{TabPack}$ } & {\footnotesize$0.9522 \pm 0.0012$} \\ 
{\footnotesize $\mathrm{MLP^\dagger}$ } & {\footnotesize$0.9627 \pm 0.0007$} \\ 
{\footnotesize $\mathrm{XGBoost}$ } & {\footnotesize$0.9606 \pm 0.0001$} \\ 
{\footnotesize $\mathrm{TabM}$ } & {\footnotesize$0.9652 \pm 0.0004$} \\ 
{\footnotesize MLP$_\text{HPE}^\dagger$ } & {\footnotesize$0.9643 \pm 0.0002$} \\ 
{\footnotesize $\mathrm{\method_\text{Offline}^\dagger}$ } & {\footnotesize$0.9643 \pm 0.0002$} \\ 
{\footnotesize $\mathrm{TabM^\dagger}$ } & {\footnotesize$0.9644 \pm 0.0007$} \\ 
{\footnotesize $\mathrm{TabPack^\dagger}$ } & {\footnotesize$0.9644 \pm 0.0003$} \\ 
\bottomrule
\end{tabular}}

&

\topalign{
\setlength\tabcolsep{2.5pt}

\begin{tabular}{lll}

\multicolumn{2}{c}{Cooking-Time \textdownarrow} \\
\toprule
Method & Single model \\
\midrule\\[-0.45cm]
{\footnotesize $\mathrm{MLP}$ } & {\footnotesize$0.4824 \pm 0.0002$} \\ 
{\footnotesize $\mathrm{TabPack}$ } & {\footnotesize$0.4810 \pm 0.0002$} \\ 
{\footnotesize $\mathrm{MLP^\dagger}$ } & {\footnotesize$0.4810 \pm 0.0001$} \\ 
{\footnotesize $\mathrm{XGBoost}$ } & {\footnotesize$0.4824 \pm 0.0001$} \\ 
{\footnotesize $\mathrm{TabM}$ } & {\footnotesize$0.4807 \pm 0.0002$} \\ 
{\footnotesize MLP$_\text{HPE}^\dagger$ } & {\footnotesize$0.4796 \pm 0.0000$} \\ 
{\footnotesize $\mathrm{\method_\text{Offline}^\dagger}$ } & {\footnotesize$0.4793 \pm 0.0001$} \\ 
{\footnotesize $\mathrm{TabM^\dagger}$ } & {\footnotesize$0.4802 \pm 0.0002$} \\ 
{\footnotesize $\mathrm{TabPack^\dagger}$ } & {\footnotesize$0.4792 \pm 0.0002$} \\ 
\bottomrule
\end{tabular}}

&

\topalign{
\setlength\tabcolsep{2.5pt}

\begin{tabular}{lll}

\multicolumn{2}{c}{Homecredit-Default \textuparrow} \\
\toprule
Method & Single model \\
\midrule\\[-0.45cm]
{\footnotesize $\mathrm{MLP}$ } & {\footnotesize$0.8551 \pm 0.0009$} \\ 
{\footnotesize $\mathrm{TabPack}$ } & {\footnotesize$0.8536 \pm 0.0008$} \\ 
{\footnotesize $\mathrm{MLP^\dagger}$ } & {\footnotesize$0.8601 \pm 0.0004$} \\ 
{\footnotesize $\mathrm{XGBoost}$ } & {\footnotesize$0.8675 \pm 0.0003$} \\ 
{\footnotesize $\mathrm{TabM}$ } & {\footnotesize$0.8613 \pm 0.0011$} \\ 
{\footnotesize MLP$_\text{HPE}^\dagger$ } & {\footnotesize$0.8620 \pm 0.0008$} \\ 
{\footnotesize $\mathrm{\method_\text{Offline}^\dagger}$ } & {\footnotesize$0.8622 \pm 0.0006$} \\ 
{\footnotesize $\mathrm{TabM^\dagger}$ } & {\footnotesize$0.8642 \pm 0.0006$} \\ 
{\footnotesize $\mathrm{TabPack^\dagger}$ } & {\footnotesize$0.8615 \pm 0.0006$} \\ 
\bottomrule
\end{tabular}}

\\

\topalign{
\setlength\tabcolsep{2.5pt}

\begin{tabular}{lll}

\multicolumn{2}{c}{Delivery-Eta \textdownarrow} \\
\toprule
Method & Single model \\
\midrule\\[-0.45cm]
{\footnotesize $\mathrm{MLP}$ } & {\footnotesize$0.5476 \pm 0.0005$} \\ 
{\footnotesize $\mathrm{TabPack}$ } & {\footnotesize$0.5499 \pm 0.0003$} \\ 
{\footnotesize $\mathrm{MLP^\dagger}$ } & {\footnotesize$0.5499 \pm 0.0008$} \\ 
{\footnotesize $\mathrm{XGBoost}$ } & {\footnotesize$0.5458 \pm 0.0001$} \\ 
{\footnotesize $\mathrm{TabM}$ } & {\footnotesize$0.5483 \pm 0.0002$} \\ 
{\footnotesize MLP$_\text{HPE}^\dagger$ } & {\footnotesize$0.5480 \pm 0.0006$} \\ 
{\footnotesize $\mathrm{\method_\text{Offline}^\dagger}$ } & {\footnotesize$0.5486 \pm 0.0007$} \\ 
{\footnotesize $\mathrm{TabM^\dagger}$ } & {\footnotesize$0.5464 \pm 0.0004$} \\ 
{\footnotesize $\mathrm{TabPack^\dagger}$ } & {\footnotesize$0.5477 \pm 0.0005$} \\ 
\bottomrule
\end{tabular}}

&

\topalign{
\setlength\tabcolsep{2.5pt}

\begin{tabular}{lll}

\multicolumn{2}{c}{Weather \textdownarrow} \\
\toprule
Method & Single model \\
\midrule\\[-0.45cm]
{\footnotesize $\mathrm{MLP}$ } & {\footnotesize$1.5010 \pm 0.0037$} \\ 
{\footnotesize $\mathrm{TabPack}$ } & {\footnotesize$1.4733 \pm 0.0010$} \\ 
{\footnotesize $\mathrm{MLP^\dagger}$ } & {\footnotesize$1.4915 \pm 0.0020$} \\ 
{\footnotesize $\mathrm{XGBoost}$ } & {\footnotesize$1.4694 \pm 0.0005$} \\ 
{\footnotesize $\mathrm{TabM}$ } & {\footnotesize$1.4651 \pm 0.0042$} \\ 
{\footnotesize MLP$_\text{HPE}^\dagger$ } & {\footnotesize$1.4616 \pm 0.0040$} \\ 
{\footnotesize $\mathrm{\method_\text{Offline}^\dagger}$ } & {\footnotesize$1.4590 \pm 0.0035$} \\ 
{\footnotesize $\mathrm{TabM^\dagger}$ } & {\footnotesize$1.4491 \pm 0.0034$} \\ 
{\footnotesize $\mathrm{TabPack^\dagger}$ } & {\footnotesize$1.4430 \pm 0.0007$} \\ 
\bottomrule
\end{tabular}}

\end{longtable}
