# Supplementary material for: TabPack: Efficient Hyperparameter Ensembles for Tabular Deep Learning
Source: arXiv:2607.05380 source file (2026-07-06)
Supplement: Supplementary file 3 [file appendix_all.tex]

\newcommand{\topalign}[1]{%
\vtop{\vskip 0pt #1}}

\begin{longtable}{p{0.5\textwidth}p{0.5\textwidth}}
\caption{
Per-dataset results for all methods evaluated in this paper. For each dataset we report the mean test score $\pm$ standard deviation over 10 random seeds.
}
\label{tab:appendix-all-results}\\

\topalign{
\centering
\setlength\tabcolsep{2.5pt}

\begin{tabular}{ll}

\multicolumn{2}{c}{\small{Churn \textuparrow}} \\
\toprule
{\small Method} & {\small Score} \\
\midrule\\[-0.7cm]
\multicolumn{2}{c}{} \\[0.05cm]
{\footnotesize $\mathrm{MLP}$ } & {\footnotesize$0.8562 \pm 0.0018$}\\ 
{\footnotesize $\mathrm{XGBoost}$ } & {\footnotesize$0.8605 \pm 0.0020$}\\ 
{\footnotesize $\mathrm{TabICLv2}$ } & {\footnotesize$0.8658 \pm 0.0008$}\\ 
{\footnotesize $\mathrm{TabPFN\texttt{-}3}$ } & {\footnotesize$0.8655 \pm 0.0009$}\\ 
{\footnotesize $\mathrm{ModernNCA^\dagger}$ } & {\footnotesize$0.8591 \pm 0.0027$}\\ 
{\footnotesize $\mathrm{RealMLP}$ } & {\footnotesize$0.8599 \pm 0.0023$}\\ 
{\footnotesize $\mathrm{TabM}$ } & {\footnotesize$0.8638 \pm 0.0017$}\\ 
{\footnotesize $\mathrm{MLP^\dagger}$ } & {\footnotesize$0.8633 \pm 0.0029$}\\ 
{\footnotesize $\mathrm{TabM^\dagger}$ } & {\footnotesize$0.8609 \pm 0.0014$}\\ 
{\footnotesize $\mathrm{TabPack}$ } & {\footnotesize$0.8575 \pm 0.0014$}\\ 
{\footnotesize $\mathrm{MLP^\dagger_{{HPE}}}$ } & {\footnotesize$0.8624 \pm 0.0013$}\\ 
{\footnotesize $\mathrm{TabPack^\dagger_{Offline}}$ } & {\footnotesize$0.8562 \pm 0.0048$}\\ 
{\footnotesize $\mathrm{TabPack^\dagger}$ } & {\footnotesize$0.8623 \pm 0.0028$}\\ 
\bottomrule
\end{tabular}}

&

\topalign{
\centering
\setlength\tabcolsep{2.5pt}

\begin{tabular}{ll}

\multicolumn{2}{c}{\small{California \textdownarrow}} \\
\toprule
{\small Method} & {\small Score} \\
\midrule\\[-0.7cm]
\multicolumn{2}{c}{} \\[0.05cm]
{\footnotesize $\mathrm{MLP}$ } & {\footnotesize$0.4819 \pm 0.0023$}\\ 
{\footnotesize $\mathrm{XGBoost}$ } & {\footnotesize$0.4329 \pm 0.0011$}\\ 
{\footnotesize $\mathrm{TabICLv2}$ } & {\footnotesize$0.3976 \pm 0.0005$}\\ 
{\footnotesize $\mathrm{TabPFN\texttt{-}3}$ } & {\footnotesize$0.3787 \pm 0.0007$}\\ 
{\footnotesize $\mathrm{ModernNCA^\dagger}$ } & {\footnotesize$0.4098 \pm 0.0035$}\\ 
{\footnotesize $\mathrm{RealMLP}$ } & {\footnotesize$0.4063 \pm 0.0011$}\\ 
{\footnotesize $\mathrm{TabM}$ } & {\footnotesize$0.4324 \pm 0.0026$}\\ 
{\footnotesize $\mathrm{MLP^\dagger}$ } & {\footnotesize$0.4376 \pm 0.0022$}\\ 
{\footnotesize $\mathrm{TabM^\dagger}$ } & {\footnotesize$0.4028 \pm 0.0019$}\\ 
{\footnotesize $\mathrm{TabPack}$ } & {\footnotesize$0.4725 \pm 0.0014$}\\ 
{\footnotesize $\mathrm{MLP^\dagger_{{HPE}}}$ } & {\footnotesize$0.4233 \pm 0.0024$}\\ 
{\footnotesize $\mathrm{TabPack^\dagger_{Offline}}$ } & {\footnotesize$0.4241 \pm 0.0025$}\\ 
{\footnotesize $\mathrm{TabPack^\dagger}$ } & {\footnotesize$0.4176 \pm 0.0028$}\\ 
\bottomrule
\end{tabular}}

\\
\topalign{
\centering
\setlength\tabcolsep{2.5pt}

\begin{tabular}{ll}

\multicolumn{2}{c}{\small{House \textdownarrow}} \\
\toprule
{\small Method} & {\small Score} \\
\midrule\\[-0.7cm]
\multicolumn{2}{c}{} \\[0.05cm]
{\footnotesize $\mathrm{MLP}$ } & {\footnotesize$30387 \pm 214$}\\ 
{\footnotesize $\mathrm{XGBoost}$ } & {\footnotesize$31381 \pm 60$}\\ 
{\footnotesize $\mathrm{TabICLv2}$ } & {\footnotesize$27958 \pm 87$}\\ 
{\footnotesize $\mathrm{TabPFN\texttt{-}3}$ } & {\footnotesize$26913 \pm 75$}\\ 
{\footnotesize $\mathrm{ModernNCA^\dagger}$ } & {\footnotesize$30713 \pm 399$}\\ 
{\footnotesize $\mathrm{RealMLP}$ } & {\footnotesize$30077 \pm 138$}\\ 
{\footnotesize $\mathrm{TabM}$ } & {\footnotesize$30390 \pm 124$}\\ 
{\footnotesize $\mathrm{MLP^\dagger}$ } & {\footnotesize$29851 \pm 411$}\\ 
{\footnotesize $\mathrm{TabM^\dagger}$ } & {\footnotesize$30151 \pm 218$}\\ 
{\footnotesize $\mathrm{TabPack}$ } & {\footnotesize$29721 \pm 91$}\\ 
{\footnotesize $\mathrm{MLP^\dagger_{{HPE}}}$ } & {\footnotesize$29611 \pm 198$}\\ 
{\footnotesize $\mathrm{TabPack^\dagger_{Offline}}$ } & {\footnotesize$29896 \pm 179$}\\ 
{\footnotesize $\mathrm{TabPack^\dagger}$ } & {\footnotesize$29549 \pm 175$}\\ 
\bottomrule
\end{tabular}}

&

\topalign{
\centering
\setlength\tabcolsep{2.5pt}

\begin{tabular}{ll}

\multicolumn{2}{c}{\small{Sberbank-Housing \textdownarrow}} \\
\toprule
{\small Method} & {\small Score} \\
\midrule\\[-0.7cm]
\multicolumn{2}{c}{} \\[0.05cm]
{\footnotesize $\mathrm{MLP}$ } & {\footnotesize$0.2608 \pm 0.0149$}\\ 
{\footnotesize $\mathrm{XGBoost}$ } & {\footnotesize$0.2407 \pm 0.0004$}\\ 
{\footnotesize $\mathrm{TabICLv2}$ } & {\footnotesize$0.3137 \pm 0.0107$}\\ 
{\footnotesize $\mathrm{TabPFN\texttt{-}3}$ } & {\footnotesize$0.2288 \pm 0.0013$}\\ 
{\footnotesize $\mathrm{ModernNCA^\dagger}$ } & {\footnotesize$0.2379 \pm 0.0047$}\\ 
{\footnotesize $\mathrm{RealMLP}$ } & {\footnotesize$0.2302 \pm 0.0012$}\\ 
{\footnotesize $\mathrm{TabM}$ } & {\footnotesize$0.2424 \pm 0.0033$}\\ 
{\footnotesize $\mathrm{MLP^\dagger}$ } & {\footnotesize$0.2481 \pm 0.0038$}\\ 
{\footnotesize $\mathrm{TabM^\dagger}$ } & {\footnotesize$0.2343 \pm 0.0013$}\\ 
{\footnotesize $\mathrm{TabPack}$ } & {\footnotesize$0.2470 \pm 0.0018$}\\ 
{\footnotesize $\mathrm{MLP^\dagger_{{HPE}}}$ } & {\footnotesize$0.2345 \pm 0.0010$}\\ 
{\footnotesize $\mathrm{TabPack^\dagger_{Offline}}$ } & {\footnotesize$0.2339 \pm 0.0023$}\\ 
{\footnotesize $\mathrm{TabPack^\dagger}$ } & {\footnotesize$0.2302 \pm 0.0014$}\\ 
\bottomrule
\end{tabular}}

\\
\topalign{
\centering
\setlength\tabcolsep{2.5pt}

\begin{tabular}{ll}

\multicolumn{2}{c}{\small{Adult \textuparrow}} \\
\toprule
{\small Method} & {\small Score} \\
\midrule\\[-0.7cm]
\multicolumn{2}{c}{} \\[0.05cm]
{\footnotesize $\mathrm{MLP}$ } & {\footnotesize$0.8561 \pm 0.0012$}\\ 
{\footnotesize $\mathrm{XGBoost}$ } & {\footnotesize$0.8709 \pm 0.0007$}\\ 
{\footnotesize $\mathrm{TabICLv2}$ } & {\footnotesize$0.8699 \pm 0.0022$}\\ 
{\footnotesize $\mathrm{TabPFN\texttt{-}3}$ } & {\footnotesize$0.8636 \pm 0.0002$}\\ 
{\footnotesize $\mathrm{ModernNCA^\dagger}$ } & {\footnotesize$0.8687 \pm 0.0011$}\\ 
{\footnotesize $\mathrm{RealMLP}$ } & {\footnotesize$0.8717 \pm 0.0014$}\\ 
{\footnotesize $\mathrm{TabM}$ } & {\footnotesize$0.8577 \pm 0.0007$}\\ 
{\footnotesize $\mathrm{MLP^\dagger}$ } & {\footnotesize$0.8692 \pm 0.0018$}\\ 
{\footnotesize $\mathrm{TabM^\dagger}$ } & {\footnotesize$0.8674 \pm 0.0010$}\\ 
{\footnotesize $\mathrm{TabPack}$ } & {\footnotesize$0.8572 \pm 0.0011$}\\ 
{\footnotesize $\mathrm{MLP^\dagger_{{HPE}}}$ } & {\footnotesize$0.8671 \pm 0.0012$}\\ 
{\footnotesize $\mathrm{TabPack^\dagger_{Offline}}$ } & {\footnotesize$0.8680 \pm 0.0023$}\\ 
{\footnotesize $\mathrm{TabPack^\dagger}$ } & {\footnotesize$0.8693 \pm 0.0007$}\\ 
\bottomrule
\end{tabular}}

&

\topalign{
\centering
\setlength\tabcolsep{2.5pt}

\begin{tabular}{ll}

\multicolumn{2}{c}{\small{Diamond \textdownarrow}} \\
\toprule
{\small Method} & {\small Score} \\
\midrule\\[-0.7cm]
\multicolumn{2}{c}{} \\[0.05cm]
{\footnotesize $\mathrm{MLP}$ } & {\footnotesize$0.1359 \pm 0.0012$}\\ 
{\footnotesize $\mathrm{XGBoost}$ } & {\footnotesize$0.1337 \pm 0.0004$}\\ 
{\footnotesize $\mathrm{TabICLv2}$ } & {\footnotesize$0.1249 \pm 0.0002$}\\ 
{\footnotesize $\mathrm{TabPFN\texttt{-}3}$ } & {\footnotesize$0.1246 \pm 0.0002$}\\ 
{\footnotesize $\mathrm{ModernNCA^\dagger}$ } & {\footnotesize$0.1331 \pm 0.0018$}\\ 
{\footnotesize $\mathrm{RealMLP}$ } & {\footnotesize$0.1308 \pm 0.0006$}\\ 
{\footnotesize $\mathrm{TabM}$ } & {\footnotesize$0.1315 \pm 0.0010$}\\ 
{\footnotesize $\mathrm{MLP^\dagger}$ } & {\footnotesize$0.1343 \pm 0.0008$}\\ 
{\footnotesize $\mathrm{TabM^\dagger}$ } & {\footnotesize$0.1306 \pm 0.0007$}\\ 
{\footnotesize $\mathrm{TabPack}$ } & {\footnotesize$0.1331 \pm 0.0003$}\\ 
{\footnotesize $\mathrm{MLP^\dagger_{{HPE}}}$ } & {\footnotesize$0.1307 \pm 0.0005$}\\ 
{\footnotesize $\mathrm{TabPack^\dagger_{Offline}}$ } & {\footnotesize$0.1309 \pm 0.0003$}\\ 
{\footnotesize $\mathrm{TabPack^\dagger}$ } & {\footnotesize$0.1307 \pm 0.0007$}\\ 
\bottomrule
\end{tabular}}

\\
\topalign{
\centering
\setlength\tabcolsep{2.5pt}

\begin{tabular}{ll}

\multicolumn{2}{c}{\small{Otto \textuparrow}} \\
\toprule
{\small Method} & {\small Score} \\
\midrule\\[-0.7cm]
\multicolumn{2}{c}{} \\[0.05cm]
{\footnotesize $\mathrm{MLP}$ } & {\footnotesize$0.8218 \pm 0.0029$}\\ 
{\footnotesize $\mathrm{XGBoost}$ } & {\footnotesize$0.8301 \pm 0.0016$}\\ 
{\footnotesize $\mathrm{TabICLv2}$ } & {\footnotesize$0.8434 \pm 0.0012$}\\ 
{\footnotesize $\mathrm{TabPFN\texttt{-}3}$ } & {\footnotesize$0.8405 \pm 0.0008$}\\ 
{\footnotesize $\mathrm{ModernNCA^\dagger}$ } & {\footnotesize$0.8298 \pm 0.0022$}\\ 
{\footnotesize $\mathrm{RealMLP}$ } & {\footnotesize$0.8287 \pm 0.0007$}\\ 
{\footnotesize $\mathrm{TabM}$ } & {\footnotesize$0.8278 \pm 0.0012$}\\ 
{\footnotesize $\mathrm{MLP^\dagger}$ } & {\footnotesize$0.8237 \pm 0.0023$}\\ 
{\footnotesize $\mathrm{TabM^\dagger}$ } & {\footnotesize$0.8332 \pm 0.0021$}\\ 
{\footnotesize $\mathrm{TabPack}$ } & {\footnotesize$0.8238 \pm 0.0012$}\\ 
{\footnotesize $\mathrm{MLP^\dagger_{{HPE}}}$ } & {\footnotesize$0.8241 \pm 0.0018$}\\ 
{\footnotesize $\mathrm{TabPack^\dagger_{Offline}}$ } & {\footnotesize$0.8248 \pm 0.0020$}\\ 
{\footnotesize $\mathrm{TabPack^\dagger}$ } & {\footnotesize$0.8281 \pm 0.0017$}\\ 
\bottomrule
\end{tabular}}

&

\topalign{
\centering
\setlength\tabcolsep{2.5pt}

\begin{tabular}{ll}

\multicolumn{2}{c}{\small{Higgs-Small \textuparrow}} \\
\toprule
{\small Method} & {\small Score} \\
\midrule\\[-0.7cm]
\multicolumn{2}{c}{} \\[0.05cm]
{\footnotesize $\mathrm{MLP}$ } & {\footnotesize$0.7267 \pm 0.0013$}\\ 
{\footnotesize $\mathrm{XGBoost}$ } & {\footnotesize$0.7271 \pm 0.0009$}\\ 
{\footnotesize $\mathrm{TabICLv2}$ } & {\footnotesize$0.7355 \pm 0.0009$}\\ 
{\footnotesize $\mathrm{TabPFN\texttt{-}3}$ } & {\footnotesize$0.7391 \pm 0.0008$}\\ 
{\footnotesize $\mathrm{ModernNCA^\dagger}$ } & {\footnotesize$0.7310 \pm 0.0014$}\\ 
{\footnotesize $\mathrm{RealMLP}$ } & {\footnotesize$0.7311 \pm 0.0014$}\\ 
{\footnotesize $\mathrm{TabM}$ } & {\footnotesize$0.7409 \pm 0.0029$}\\ 
{\footnotesize $\mathrm{MLP^\dagger}$ } & {\footnotesize$0.7279 \pm 0.0007$}\\ 
{\footnotesize $\mathrm{TabM^\dagger}$ } & {\footnotesize$0.7352 \pm 0.0008$}\\ 
{\footnotesize $\mathrm{TabPack}$ } & {\footnotesize$0.7288 \pm 0.0021$}\\ 
{\footnotesize $\mathrm{MLP^\dagger_{{HPE}}}$ } & {\footnotesize$0.7313 \pm 0.0008$}\\ 
{\footnotesize $\mathrm{TabPack^\dagger_{Offline}}$ } & {\footnotesize$0.7309 \pm 0.0007$}\\ 
{\footnotesize $\mathrm{TabPack^\dagger}$ } & {\footnotesize$0.7317 \pm 0.0010$}\\ 
\bottomrule
\end{tabular}}

\\
\topalign{
\centering
\setlength\tabcolsep{2.5pt}

\begin{tabular}{ll}

\multicolumn{2}{c}{\small{Black-Friday \textdownarrow}} \\
\toprule
{\small Method} & {\small Score} \\
\midrule\\[-0.7cm]
\multicolumn{2}{c}{} \\[0.05cm]
{\footnotesize $\mathrm{MLP}$ } & {\footnotesize$0.6927 \pm 0.0006$}\\ 
{\footnotesize $\mathrm{XGBoost}$ } & {\footnotesize$0.6808 \pm 0.0001$}\\ 
{\footnotesize $\mathrm{TabICLv2}$ } & {\footnotesize$0.6919 \pm 0.0002$}\\ 
{\footnotesize $\mathrm{TabPFN\texttt{-}3}$ } & {\footnotesize$0.7026 \pm 0.0028$}\\ 
{\footnotesize $\mathrm{ModernNCA^\dagger}$ } & {\footnotesize$0.6861 \pm 0.0006$}\\ 
{\footnotesize $\mathrm{RealMLP}$ } & {\footnotesize$0.6781 \pm 0.0004$}\\ 
{\footnotesize $\mathrm{TabM}$ } & {\footnotesize$0.6846 \pm 0.0003$}\\ 
{\footnotesize $\mathrm{MLP^\dagger}$ } & {\footnotesize$0.6816 \pm 0.0006$}\\ 
{\footnotesize $\mathrm{TabM^\dagger}$ } & {\footnotesize$0.6766 \pm 0.0006$}\\ 
{\footnotesize $\mathrm{TabPack}$ } & {\footnotesize$0.6877 \pm 0.0003$}\\ 
{\footnotesize $\mathrm{MLP^\dagger_{{HPE}}}$ } & {\footnotesize$0.6802 \pm 0.0003$}\\ 
{\footnotesize $\mathrm{TabPack^\dagger_{Offline}}$ } & {\footnotesize$0.6797 \pm 0.0005$}\\ 
{\footnotesize $\mathrm{TabPack^\dagger}$ } & {\footnotesize$0.6784 \pm 0.0002$}\\ 
\bottomrule
\end{tabular}}

&

\topalign{
\centering
\setlength\tabcolsep{2.5pt}

\begin{tabular}{ll}

\multicolumn{2}{c}{\small{Ecom-Offers \textuparrow}} \\
\toprule
{\small Method} & {\small Score} \\
\midrule\\[-0.7cm]
\multicolumn{2}{c}{} \\[0.05cm]
{\footnotesize $\mathrm{MLP}$ } & {\footnotesize$0.6011 \pm 0.0025$}\\ 
{\footnotesize $\mathrm{XGBoost}$ } & {\footnotesize$0.5741 \pm 0.0055$}\\ 
{\footnotesize $\mathrm{TabICLv2}$ } & {\footnotesize$0.5974 \pm 0.0020$}\\ 
{\footnotesize $\mathrm{TabPFN\texttt{-}3}$ } & {\footnotesize$0.6343 \pm 0.0009$}\\ 
{\footnotesize $\mathrm{ModernNCA^\dagger}$ } & {\footnotesize$0.5831 \pm 0.0019$}\\ 
{\footnotesize $\mathrm{RealMLP}$ } & {\footnotesize$0.5806 \pm 0.0145$}\\ 
{\footnotesize $\mathrm{TabM}$ } & {\footnotesize$0.6016 \pm 0.0004$}\\ 
{\footnotesize $\mathrm{MLP^\dagger}$ } & {\footnotesize$0.5993 \pm 0.0008$}\\ 
{\footnotesize $\mathrm{TabM^\dagger}$ } & {\footnotesize$0.5984 \pm 0.0010$}\\ 
{\footnotesize $\mathrm{TabPack}$ } & {\footnotesize$0.6018 \pm 0.0012$}\\ 
{\footnotesize $\mathrm{MLP^\dagger_{{HPE}}}$ } & {\footnotesize$0.5986 \pm 0.0017$}\\ 
{\footnotesize $\mathrm{TabPack^\dagger_{Offline}}$ } & {\footnotesize$0.5987 \pm 0.0009$}\\ 
{\footnotesize $\mathrm{TabPack^\dagger}$ } & {\footnotesize$0.5989 \pm 0.0017$}\\ 
\bottomrule
\end{tabular}}

\\
\topalign{
\centering
\setlength\tabcolsep{2.5pt}

\begin{tabular}{ll}

\multicolumn{2}{c}{\small{Maps-Routing \textdownarrow}} \\
\toprule
{\small Method} & {\small Score} \\
\midrule\\[-0.7cm]
\multicolumn{2}{c}{} \\[0.05cm]
{\footnotesize $\mathrm{MLP}$ } & {\footnotesize$0.1622 \pm 0.0001$}\\ 
{\footnotesize $\mathrm{XGBoost}$ } & {\footnotesize$0.1618 \pm 0.0000$}\\ 
{\footnotesize $\mathrm{TabICLv2}$ } & {\footnotesize$0.1657 \pm 0.0002$}\\ 
{\footnotesize $\mathrm{TabPFN\texttt{-}3}$ } & {\footnotesize$0.1643 \pm 0.0002$}\\ 
{\footnotesize $\mathrm{ModernNCA^\dagger}$ } & {\footnotesize$0.1628 \pm 0.0000$}\\ 
{\footnotesize $\mathrm{RealMLP}$ } & {\footnotesize$0.1609 \pm 0.0001$}\\ 
{\footnotesize $\mathrm{TabM}$ } & {\footnotesize$0.1611 \pm 0.0001$}\\ 
{\footnotesize $\mathrm{MLP^\dagger}$ } & {\footnotesize$0.1612 \pm 0.0001$}\\ 
{\footnotesize $\mathrm{TabM^\dagger}$ } & {\footnotesize$0.1606 \pm 0.0002$}\\ 
{\footnotesize $\mathrm{TabPack}$ } & {\footnotesize$0.1612 \pm 0.0000$}\\ 
{\footnotesize $\mathrm{MLP^\dagger_{{HPE}}}$ } & {\footnotesize$0.1607 \pm 0.0001$}\\ 
{\footnotesize $\mathrm{TabPack^\dagger_{Offline}}$ } & {\footnotesize$0.1610 \pm 0.0001$}\\ 
{\footnotesize $\mathrm{TabPack^\dagger}$ } & {\footnotesize$0.1605 \pm 0.0001$}\\ 
\bottomrule
\end{tabular}}

&

\topalign{
\centering
\setlength\tabcolsep{2.5pt}

\begin{tabular}{ll}

\multicolumn{2}{c}{\small{Homesite-Insurance \textuparrow}} \\
\toprule
{\small Method} & {\small Score} \\
\midrule\\[-0.7cm]
\multicolumn{2}{c}{} \\[0.05cm]
{\footnotesize $\mathrm{MLP}$ } & {\footnotesize$0.9515 \pm 0.0007$}\\ 
{\footnotesize $\mathrm{XGBoost}$ } & {\footnotesize$0.9606 \pm 0.0001$}\\ 
{\footnotesize $\mathrm{TabICLv2}$ } & {\footnotesize$0.9470 \pm 0.0046$}\\ 
{\footnotesize $\mathrm{TabPFN\texttt{-}3}$ } & {\footnotesize$0.9568 \pm 0.0015$}\\ 
{\footnotesize $\mathrm{ModernNCA^\dagger}$ } & {\footnotesize$0.9629 \pm 0.0003$}\\ 
{\footnotesize $\mathrm{RealMLP}$ } & {\footnotesize$0.9600 \pm 0.0015$}\\ 
{\footnotesize $\mathrm{TabM}$ } & {\footnotesize$0.9652 \pm 0.0004$}\\ 
{\footnotesize $\mathrm{MLP^\dagger}$ } & {\footnotesize$0.9627 \pm 0.0007$}\\ 
{\footnotesize $\mathrm{TabM^\dagger}$ } & {\footnotesize$0.9644 \pm 0.0007$}\\ 
{\footnotesize $\mathrm{TabPack}$ } & {\footnotesize$0.9518 \pm 0.0002$}\\ 
{\footnotesize $\mathrm{MLP^\dagger_{{HPE}}}$ } & {\footnotesize$0.9638 \pm 0.0004$}\\ 
{\footnotesize $\mathrm{TabPack^\dagger_{Offline}}$ } & {\footnotesize$0.9640 \pm 0.0004$}\\ 
{\footnotesize $\mathrm{TabPack^\dagger}$ } & {\footnotesize$0.9644 \pm 0.0003$}\\ 
\bottomrule
\end{tabular}}

\\
\topalign{
\centering
\setlength\tabcolsep{2.5pt}

\begin{tabular}{ll}

\multicolumn{2}{c}{\small{Cooking-Time \textdownarrow}} \\
\toprule
{\small Method} & {\small Score} \\
\midrule\\[-0.7cm]
\multicolumn{2}{c}{} \\[0.05cm]
{\footnotesize $\mathrm{MLP}$ } & {\footnotesize$0.4824 \pm 0.0002$}\\ 
{\footnotesize $\mathrm{XGBoost}$ } & {\footnotesize$0.4824 \pm 0.0001$}\\ 
{\footnotesize $\mathrm{TabICLv2}$ } & {\footnotesize$0.4851 \pm 0.0004$}\\ 
{\footnotesize $\mathrm{TabPFN\texttt{-}3}$ } & {\footnotesize$0.4844 \pm 0.0004$}\\ 
{\footnotesize $\mathrm{ModernNCA^\dagger}$ } & {\footnotesize$0.4813 \pm 0.0003$}\\ 
{\footnotesize $\mathrm{RealMLP}$ } & {\footnotesize$0.4809 \pm 0.0005$}\\ 
{\footnotesize $\mathrm{TabM}$ } & {\footnotesize$0.4807 \pm 0.0002$}\\ 
{\footnotesize $\mathrm{MLP^\dagger}$ } & {\footnotesize$0.4810 \pm 0.0001$}\\ 
{\footnotesize $\mathrm{TabM^\dagger}$ } & {\footnotesize$0.4802 \pm 0.0002$}\\ 
{\footnotesize $\mathrm{TabPack}$ } & {\footnotesize$0.4810 \pm 0.0000$}\\ 
{\footnotesize $\mathrm{MLP^\dagger_{{HPE}}}$ } & {\footnotesize$0.4795 \pm 0.0003$}\\ 
{\footnotesize $\mathrm{TabPack^\dagger_{Offline}}$ } & {\footnotesize$0.4798 \pm 0.0002$}\\ 
{\footnotesize $\mathrm{TabPack^\dagger}$ } & {\footnotesize$0.4792 \pm 0.0002$}\\ 
\bottomrule
\end{tabular}}

&

\topalign{
\centering
\setlength\tabcolsep{2.5pt}

\begin{tabular}{ll}

\multicolumn{2}{c}{\small{Homecredit-Default \textuparrow}} \\
\toprule
{\small Method} & {\small Score} \\
\midrule\\[-0.7cm]
\multicolumn{2}{c}{} \\[0.05cm]
{\footnotesize $\mathrm{MLP}$ } & {\footnotesize$0.8551 \pm 0.0009$}\\ 
{\footnotesize $\mathrm{XGBoost}$ } & {\footnotesize$0.8675 \pm 0.0003$}\\ 
{\footnotesize $\mathrm{TabICLv2}$ } & {\footnotesize$0.8454 \pm 0.0019$}\\ 
{\footnotesize $\mathrm{TabPFN\texttt{-}3}$ } & {\footnotesize$0.8501 \pm 0.0014$}\\ 
{\footnotesize $\mathrm{ModernNCA^\dagger}$ } & {\footnotesize$0.8526 \pm 0.0019$}\\ 
{\footnotesize $\mathrm{RealMLP}$ } & {\footnotesize$0.8509 \pm 0.0023$}\\ 
{\footnotesize $\mathrm{TabM}$ } & {\footnotesize$0.8613 \pm 0.0011$}\\ 
{\footnotesize $\mathrm{MLP^\dagger}$ } & {\footnotesize$0.8601 \pm 0.0004$}\\ 
{\footnotesize $\mathrm{TabM^\dagger}$ } & {\footnotesize$0.8642 \pm 0.0006$}\\ 
{\footnotesize $\mathrm{TabPack}$ } & {\footnotesize$0.8535 \pm 0.0003$}\\ 
{\footnotesize $\mathrm{MLP^\dagger_{{HPE}}}$ } & {\footnotesize$0.8615 \pm 0.0015$}\\ 
{\footnotesize $\mathrm{TabPack^\dagger_{Offline}}$ } & {\footnotesize$0.8617 \pm 0.0010$}\\ 
{\footnotesize $\mathrm{TabPack^\dagger}$ } & {\footnotesize$0.8615 \pm 0.0006$}\\ 
\bottomrule
\end{tabular}}

\\
\topalign{
\centering
\setlength\tabcolsep{2.5pt}

\begin{tabular}{ll}

\multicolumn{2}{c}{\small{Delivery-Eta \textdownarrow}} \\
\toprule
{\small Method} & {\small Score} \\
\midrule\\[-0.7cm]
\multicolumn{2}{c}{} \\[0.05cm]
{\footnotesize $\mathrm{MLP}$ } & {\footnotesize$0.5476 \pm 0.0005$}\\ 
{\footnotesize $\mathrm{XGBoost}$ } & {\footnotesize$0.5458 \pm 0.0001$}\\ 
{\footnotesize $\mathrm{TabICLv2}$ } & {\footnotesize$0.5537 \pm 0.0003$}\\ 
{\footnotesize $\mathrm{TabPFN\texttt{-}3}$ } & {\footnotesize$0.5545 \pm 0.0009$}\\ 
{\footnotesize $\mathrm{ModernNCA^\dagger}$ } & {\footnotesize$0.5508 \pm 0.0003$}\\ 
{\footnotesize $\mathrm{RealMLP}$ } & {\footnotesize$0.5468 \pm 0.0009$}\\ 
{\footnotesize $\mathrm{TabM}$ } & {\footnotesize$0.5483 \pm 0.0002$}\\ 
{\footnotesize $\mathrm{MLP^\dagger}$ } & {\footnotesize$0.5499 \pm 0.0008$}\\ 
{\footnotesize $\mathrm{TabM^\dagger}$ } & {\footnotesize$0.5464 \pm 0.0004$}\\ 
{\footnotesize $\mathrm{TabPack}$ } & {\footnotesize$0.5502 \pm 0.0004$}\\ 
{\footnotesize $\mathrm{MLP^\dagger_{{HPE}}}$ } & {\footnotesize$0.5490 \pm 0.0009$}\\ 
{\footnotesize $\mathrm{TabPack^\dagger_{Offline}}$ } & {\footnotesize$0.5486 \pm 0.0009$}\\ 
{\footnotesize $\mathrm{TabPack^\dagger}$ } & {\footnotesize$0.5477 \pm 0.0005$}\\ 
\bottomrule
\end{tabular}}

&

\topalign{
\centering
\setlength\tabcolsep{2.5pt}

\begin{tabular}{ll}

\multicolumn{2}{c}{\small{Weather \textdownarrow}} \\
\toprule
{\small Method} & {\small Score} \\
\midrule\\[-0.7cm]
\multicolumn{2}{c}{} \\[0.05cm]
{\footnotesize $\mathrm{MLP}$ } & {\footnotesize$1.5010 \pm 0.0037$}\\ 
{\footnotesize $\mathrm{XGBoost}$ } & {\footnotesize$1.4694 \pm 0.0005$}\\ 
{\footnotesize $\mathrm{TabICLv2}$ } & {\footnotesize$1.4690 \pm 0.0029$}\\ 
{\footnotesize $\mathrm{TabPFN\texttt{-}3}$ } & {\footnotesize$1.4597 \pm 0.0011$}\\ 
{\footnotesize $\mathrm{ModernNCA^\dagger}$ } & {\footnotesize$1.5007 \pm 0.0028$}\\ 
{\footnotesize $\mathrm{RealMLP}$ } & {\footnotesize$1.4398 \pm 0.0016$}\\ 
{\footnotesize $\mathrm{TabM}$ } & {\footnotesize$1.4651 \pm 0.0042$}\\ 
{\footnotesize $\mathrm{MLP^\dagger}$ } & {\footnotesize$1.4915 \pm 0.0020$}\\ 
{\footnotesize $\mathrm{TabM^\dagger}$ } & {\footnotesize$1.4491 \pm 0.0034$}\\ 
{\footnotesize $\mathrm{TabPack}$ } & {\footnotesize$1.4742 \pm 0.0010$}\\ 
{\footnotesize $\mathrm{MLP^\dagger_{{HPE}}}$ } & {\footnotesize$1.4607 \pm 0.0021$}\\ 
{\footnotesize $\mathrm{TabPack^\dagger_{Offline}}$ } & {\footnotesize$1.4659 \pm 0.0040$}\\ 
{\footnotesize $\mathrm{TabPack^\dagger}$ } & {\footnotesize$1.4430 \pm 0.0007$}\\ 
\bottomrule
\end{tabular}}

\\
\topalign{
\centering
\setlength\tabcolsep{2.5pt}

\begin{tabular}{ll}

\multicolumn{2}{c}{\small{Microsoft \textdownarrow}} \\
\toprule
{\small Method} & {\small Score} \\
\midrule\\[-0.7cm]
\multicolumn{2}{c}{} \\[0.05cm]
{\footnotesize $\mathrm{MLP}$ } & {\footnotesize$0.7455 \pm 0.0003$}\\ 
{\footnotesize $\mathrm{XGBoost}$ } & {\footnotesize$0.7412 \pm 0.0001$}\\ 
{\footnotesize $\mathrm{TabICLv2}$ } & {\footnotesize$0.7457 \pm 0.0002$}\\ 
{\footnotesize $\mathrm{TabPFN\texttt{-}3}$ } & {\footnotesize$0.7785 \pm 0.0026$}\\ 
{\footnotesize $\mathrm{ModernNCA^\dagger}$ } & {\footnotesize$0.7443 \pm 0.0005$}\\ 
{\footnotesize $\mathrm{RealMLP}$ } & {\footnotesize$0.7446 \pm 0.0009$}\\ 
{\footnotesize $\mathrm{TabM}$ } & {\footnotesize$0.7422 \pm 0.0004$}\\ 
{\footnotesize $\mathrm{MLP^\dagger}$ } & {\footnotesize$0.7447 \pm 0.0002$}\\ 
{\footnotesize $\mathrm{TabM^\dagger}$ } & {\footnotesize$0.7407 \pm 0.0002$}\\ 
{\footnotesize $\mathrm{TabPack}$ } & {\footnotesize$0.7423 \pm 0.0002$}\\ 
{\footnotesize $\mathrm{MLP^\dagger_{{HPE}}}$ } & {\footnotesize$0.7421 \pm 0.0005$}\\ 
{\footnotesize $\mathrm{TabPack^\dagger_{Offline}}$ } & {\footnotesize$0.7424 \pm 0.0002$}\\ 
{\footnotesize $\mathrm{TabPack^\dagger}$ } & {\footnotesize$0.7395 \pm 0.0002$}\\ 
\bottomrule
\end{tabular}}

& 

\\

\end{longtable}
